# Supplementary material for: Query-Conditioned Spherical Centroid Aggregation for Multimodal Retrieval
Source: arXiv:2609.15335 source file (2026-09-14)
Supplement: Supplementary file 1 [file table3_supp_twostage.tex]

\begin{table}[t]
\centering
\caption{Two-stage (reranked) R@1 on the identical masked cells of Table~3, with each method's own video-only cosine at $r{=}90\%$. The reranker -- one frozen cross-encoder shared by all methods, trained only on complete pairs -- converges every method onto its video pathway as $r$ grows, erasing the aggregator differences of Table~3: end-to-end robustness in a two-stage pipeline is capped by the shared reranker, which is why the main table reports the representation stage.}
\label{tab:missing_twostage}
\small
\setlength{\tabcolsep}{4.5pt}
\begin{tabular}{llcccccc}
\toprule
 & Method & 0\% & 25\% & 50\% & 75\% & 90\% & cos$_{TV}$@90\% \\
\midrule
MSR-VTT & \textbf{SCA} (ours) & \textbf{54.8} & \textbf{47.8} & \textbf{41.1} & \textbf{37.0} & \textbf{33.2} & 32.1 \\
 & GRAM$^{\star}$ & 52.5 & 47.0 & 40.9 & 35.4 & 32.9 & 32.8 \\
\rowcolor{gray!10} & \emph{margin} & +2.3 & +0.8 & +0.2 & +1.6 & +0.3 &  \\
\midrule
DiDeMo & \textbf{SCA} (ours) & \textbf{51.3} & 44.2 & 38.9 & 32.1 & 29.5 & 23.2 \\
 & \gram{}$^{\star}$ & 50.7 & \textbf{45.0} & \textbf{39.8} & \textbf{32.7} & \textbf{29.8} & 21.1 \\
\rowcolor{gray!10} & \emph{margin} & +0.6 & -0.8 & -0.9 & -0.6 & -0.3 &  \\
\midrule
ActivityNet & \textbf{SCA} (ours) & 55.8 & 47.9 & 40.0 & 33.8 & 30.7 & 23.7 \\
 & \gram{}$^{\star}$ & \textbf{56.3} & \textbf{48.3} & \textbf{41.4} & \textbf{35.5} & \textbf{32.3} & 24.8 \\
\rowcolor{gray!10} & \emph{margin} & -0.5 & -0.4 & -1.4 & -1.7 & -1.6 &  \\
\midrule
VATEX & \textbf{SCA} (ours) & \textbf{90.5} & \textbf{85.2} & \textbf{73.3} & \textbf{61.9} & 57.3 & 58.5 \\
 & \gram{}$^{\star}$ & 90.0 & 82.8 & 72.9 & \textbf{61.9} & \textbf{57.8} & 58.0 \\
\rowcolor{gray!10} & \emph{margin} & +0.5 & +2.4 & +0.4 & +0.0 & -0.5 &  \\
\midrule
AudioCaps & \textbf{SCA} (ours) & \textbf{35.2} & 24.6 & 19.2 & 13.2 & 9.9 & 10.2 \\
 & \gram{}$^{\star}$ & 32.2 & \textbf{26.0} & \textbf{21.0} & \textbf{15.5} & \textbf{11.4} & 9.5 \\
\rowcolor{gray!10} & \emph{margin} & +3.0 & -1.4 & -1.8 & -2.3 & -1.5 &  \\
\bottomrule
\end{tabular}
\end{table}
